# Supplementary material for: Task-Agnostic Language Model Watermarking via High Entropy Passthrough Layers
Source: arXiv:2412.12563 source file (2024-12-17)
Supplement: Supplementary file 1 [file table_bl_comp_additional_results.tex]

\begin{table*}
    \centering
    \small
    \caption{Additional results for passthrough watermarking against baseline methods. }
    \label{table:bl-comp-additional}
    \begin{tabular}{cclllll}
        \toprule
        Task & \parbox{1cm}{Dataset} & Method & ACC $\uparrow$ & WACC $\uparrow$ & FP $\downarrow$ & Runtime (hr) $\downarrow$ \\
        \midrule
             \multirow[c]{4}{*}{\parbox{1.25cm}{\centering  Sentiment  \\ Detection}}  
             & \multirow{2}{*}{IMDB} & PTL-1                            & 0.937 & 0.994 & 0.004 & \alert{X} \\
             &                       & PTL-135                          & 0.940 & 0.994 & 0.005 & \alert{X} \\
        \cmidrule(lr){2-7}
             & \multirow{2}{*}{SST2} & PTL-1                            & 0.919 & 1.000 & 0.000 & \alert{X} \\
             &                       & PTL-135                          & 0.921 & 1.000 & 0.003 & \alert{X} \\
             \midrule
                  \multirow[c]{4}{*}{\parbox{1.25cm}{\centering  Entailment \\ Detection}}   
                  & \multirow{2}{*}{MNLI} & PTL-1                            & 0.890 & 0.981 & 0.014 & \alert{X} \\
                  &                       & PTL-135                          & 0.889 & 0.982 & 0.017 & \alert{X} \\
             \cmidrule(lr){2-7}
                  & \multirow{2}{*}{SNLI} & PTL-1                            & 0.922 & 0.985 & 0.034 & \alert{X} \\
                  &                       & PTL-135                          & 0.921 & 0.982 & 0.037 & \alert{X} \\
             \midrule
                  \multirow[c]{4}{*}{\parbox{1.25cm}{\centering  Topic \\ Detection}}    
                  & \multirow{2}{*}{AG News} & PTL-1                            & 0.994 & 0.996 & 0.001 & \alert{X} \\
                  &                        & PTL-135                          & 0.994 & 1.000 & 0.001 & \alert{X} \\
        \cmidrule(lr){2-7}
            & \multirow{2}{*}{Newsgroup} & PTL-1                       & 0.991 & 0.799 & 0.027 & \alert{X} \\
            &                       & PTL-135                     & 0.990 & 0.836 & 0.016 & \alert{X} \\
            \midrule
            \multirow[c]{2}{*}{\parbox{1.25cm}{\centering  Paraphrase\\Detection}}     
            & \multirow{2}{*}{PAWS} & PTL-1                       & 0.880 & 0.859 & 0.211 & \alert{X} \\
                &                       & PTL-135                     & 0.901 & 0.944 & 0.031 & \alert{X} \\
                 \bottomrule
             \end{tabular}
    \end{table*}
